# Supplementary material for: MonoGS++: Fast and Accurate Monocular RGB Gaussian SLAM
Source: arXiv:2504.02437 source file (2025-04-03)
Supplement: Supplementary file 1 [file supp_rgbd.tex]

\begin{table}[htbp]
\centering
\resizebox{0.9\textwidth}{!}{
\begin{tabular}{ccccccccc}
\hline
Method        & Modality & Metric                   & room2 & office2 & office4 & fr1/desk2                     & fr2/xyz                       & fr3/office                     \\ \hline
MonoGS        & RGB      & PSNR{[}dB{]}$\uparrow$   & 31.82 & 27.01   & 27.29   & 14.06                         & 22.06                         & 23.02 \\
              &          & SSIM$\uparrow$           & 0.92  & 0.88    & 0.90    & 0.50                          & 0.72                          & 0.78                           \\
              &          & LPIPS$\downarrow$        & 0.16  & 0.26    & 0.25    & 0.62                          & 0.27                          & 0.32                           \\
              &          & ATE-MSE (cm)$\downarrow$ & 6.53  & 20.89   & 43.85   & 79.45                         & 4.31                          & 1.85  \\ \hline
MonoGS        & RGB-D    & PSNR{[}dB{]}$\uparrow$   & \underline{37.49} & \underline{36.24}   & 37.06   & 8.90                          & 12.46                         & 15.95                          \\
              &          & SSIM$\uparrow$           & \underline{0.96}  & \textbf{0.96}    & \underline{0.95}    & 0.31                          & 0.71                          & 0.46                           \\
              &          & LPIPS$\downarrow$        & 0.075 & \textbf{0.078}   & 0.099   & 0.71                          & 0.30                          & 0.74                           \\
              &          & ATE-MSE (cm)$\downarrow$ & 0.31  & \textbf{0.31}    & 3.2     & 90.92                         & 1.47                          & 104.88                         \\ \hline
\textbf{Ours} & RGB      & PSNR{[}dB{]}$\uparrow$   & 37.01 & 36.11   & 37.28   & \underline{20.64}                & \underline{26.52}                & \underline{25.08}                 \\
              &          & SSIM$\uparrow$           & \underline{0.96}  & \underline{0.95}    & \textbf{0.96}    & \underline{0.77} & \underline{0.86} & \underline{0.85}                  \\
              &          & LPIPS$\downarrow$        & \underline{0.077} & 0.090   & \underline{0.086}   & \underline{0.29}                 & \underline{0.13}                 & \underline{0.18}                  \\
              &          & ATE-MSE (cm)$\downarrow$ & \underline{0.22}  & 0.42    & \underline{0.42}    & \underline{5.18}                          & \textbf{0.38}                 & \underline{0.36}                  \\ \hline
\textbf{Ours}          & RGB-D    & PSNR{[}dB{]}$\uparrow$   & \textbf{38.25} & \textbf{36.43}   & \textbf{38.11}   & \textbf{21.70}                         & \textbf{27.08}                         & \textbf{25.79}                          \\
              &          & SSIM$\uparrow$           & \textbf{0.97}  & \textbf{0.96}    & \textbf{0.96}    & \textbf{0.79}                          & \textbf{0.87}                          & \textbf{0.86}                           \\
              &          & LPIPS$\downarrow$        & \textbf{0.075} & \underline{0.081}   & \textbf{0.084}   & \textbf{0.252}                         & \textbf{0.113}                         & \textbf{0.169 }                         \\
              &          & ATE-MSE (cm)$\downarrow$ & \textbf{0.19}  & \underline{0.32}    & \textbf{0.40}    & \textbf{4.66}                          & \underline{0.42}                          & \textbf{0.31}        \\ \hline  
\end{tabular}
}
\caption{\textbf{Comparison with MonoGS~\cite{monogs}.} We conduct experiments both taking monocular RGB and RGB-D as input on Replica~\cite{replica} and TUM-RGBD~\cite{tum-rgbd} datasets, each consisting of 3 sequences. The best results are shown in \textbf{bold}, and the second best results are \underline{underlined}.}
\label{tab:tab_rgbd}
\end{table}
