# Supplementary material for: MonoGS++: Fast and Accurate Monocular RGB Gaussian SLAM
Source: arXiv:2504.02437 source file (2025-04-03)
Supplement: Supplementary file 2 [file supp_clarity.tex]

\begin{figure*}[ht]
    \centering
    \includegraphics[width=0.95\textwidth]{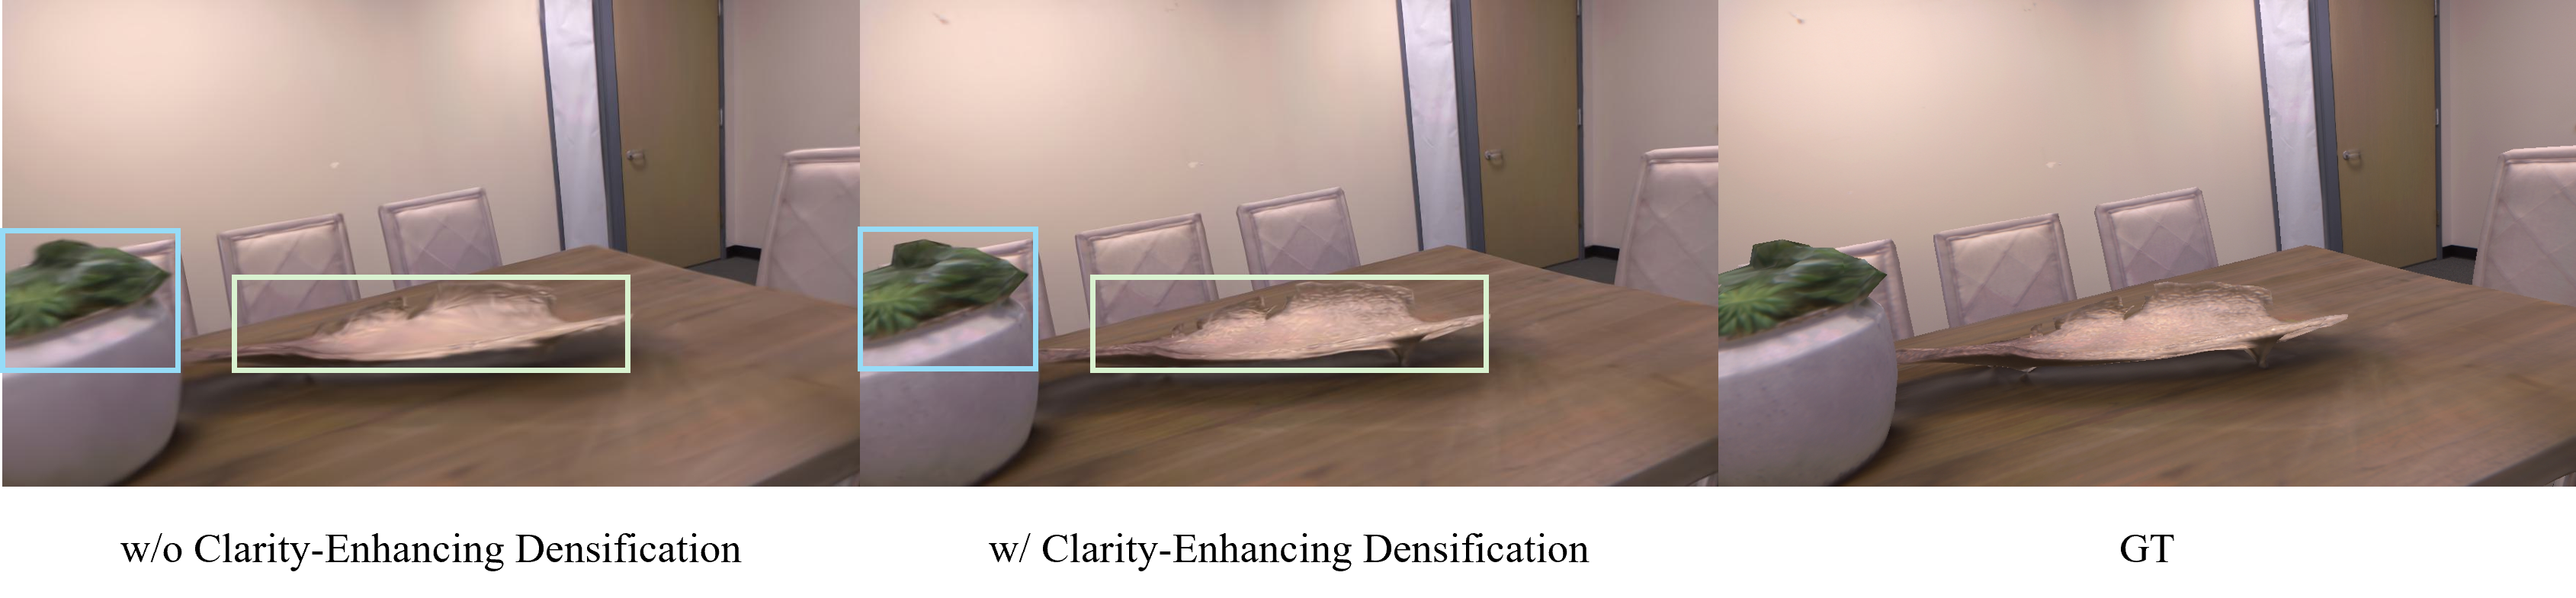}
    \caption{Visual comparison results of with and without Clarity-Enhancing Densification.}
    \label{fig:fig_supp_clarity}
\end{figure*}
