# Supplementary material for: MonoGS++: Fast and Accurate Monocular RGB Gaussian SLAM
Source: arXiv:2504.02437 source file (2025-04-03)
Supplement: Supplementary file 3 [file supp_plane.tex]

\begin{figure*}[ht]
    \centering
    \includegraphics[width=0.85\textwidth]{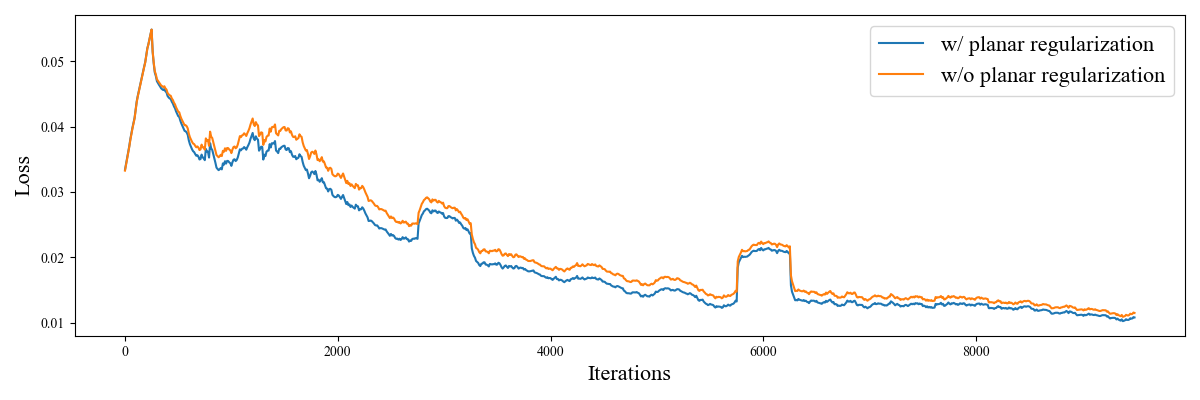}
    \caption{Loss curve of our method with and without planar regularization.}
    \label{fig:fig_supp_plane}
\end{figure*}
