# Supplementary material for: MonoGS++: Fast and Accurate Monocular RGB Gaussian SLAM
Source: arXiv:2504.02437 source file (2025-04-03)
Supplement: Supplementary file 5 [file supp_vis2.tex]

\begin{figure*}[htbp]
    \centering
    \includegraphics[width=0.95\textwidth]{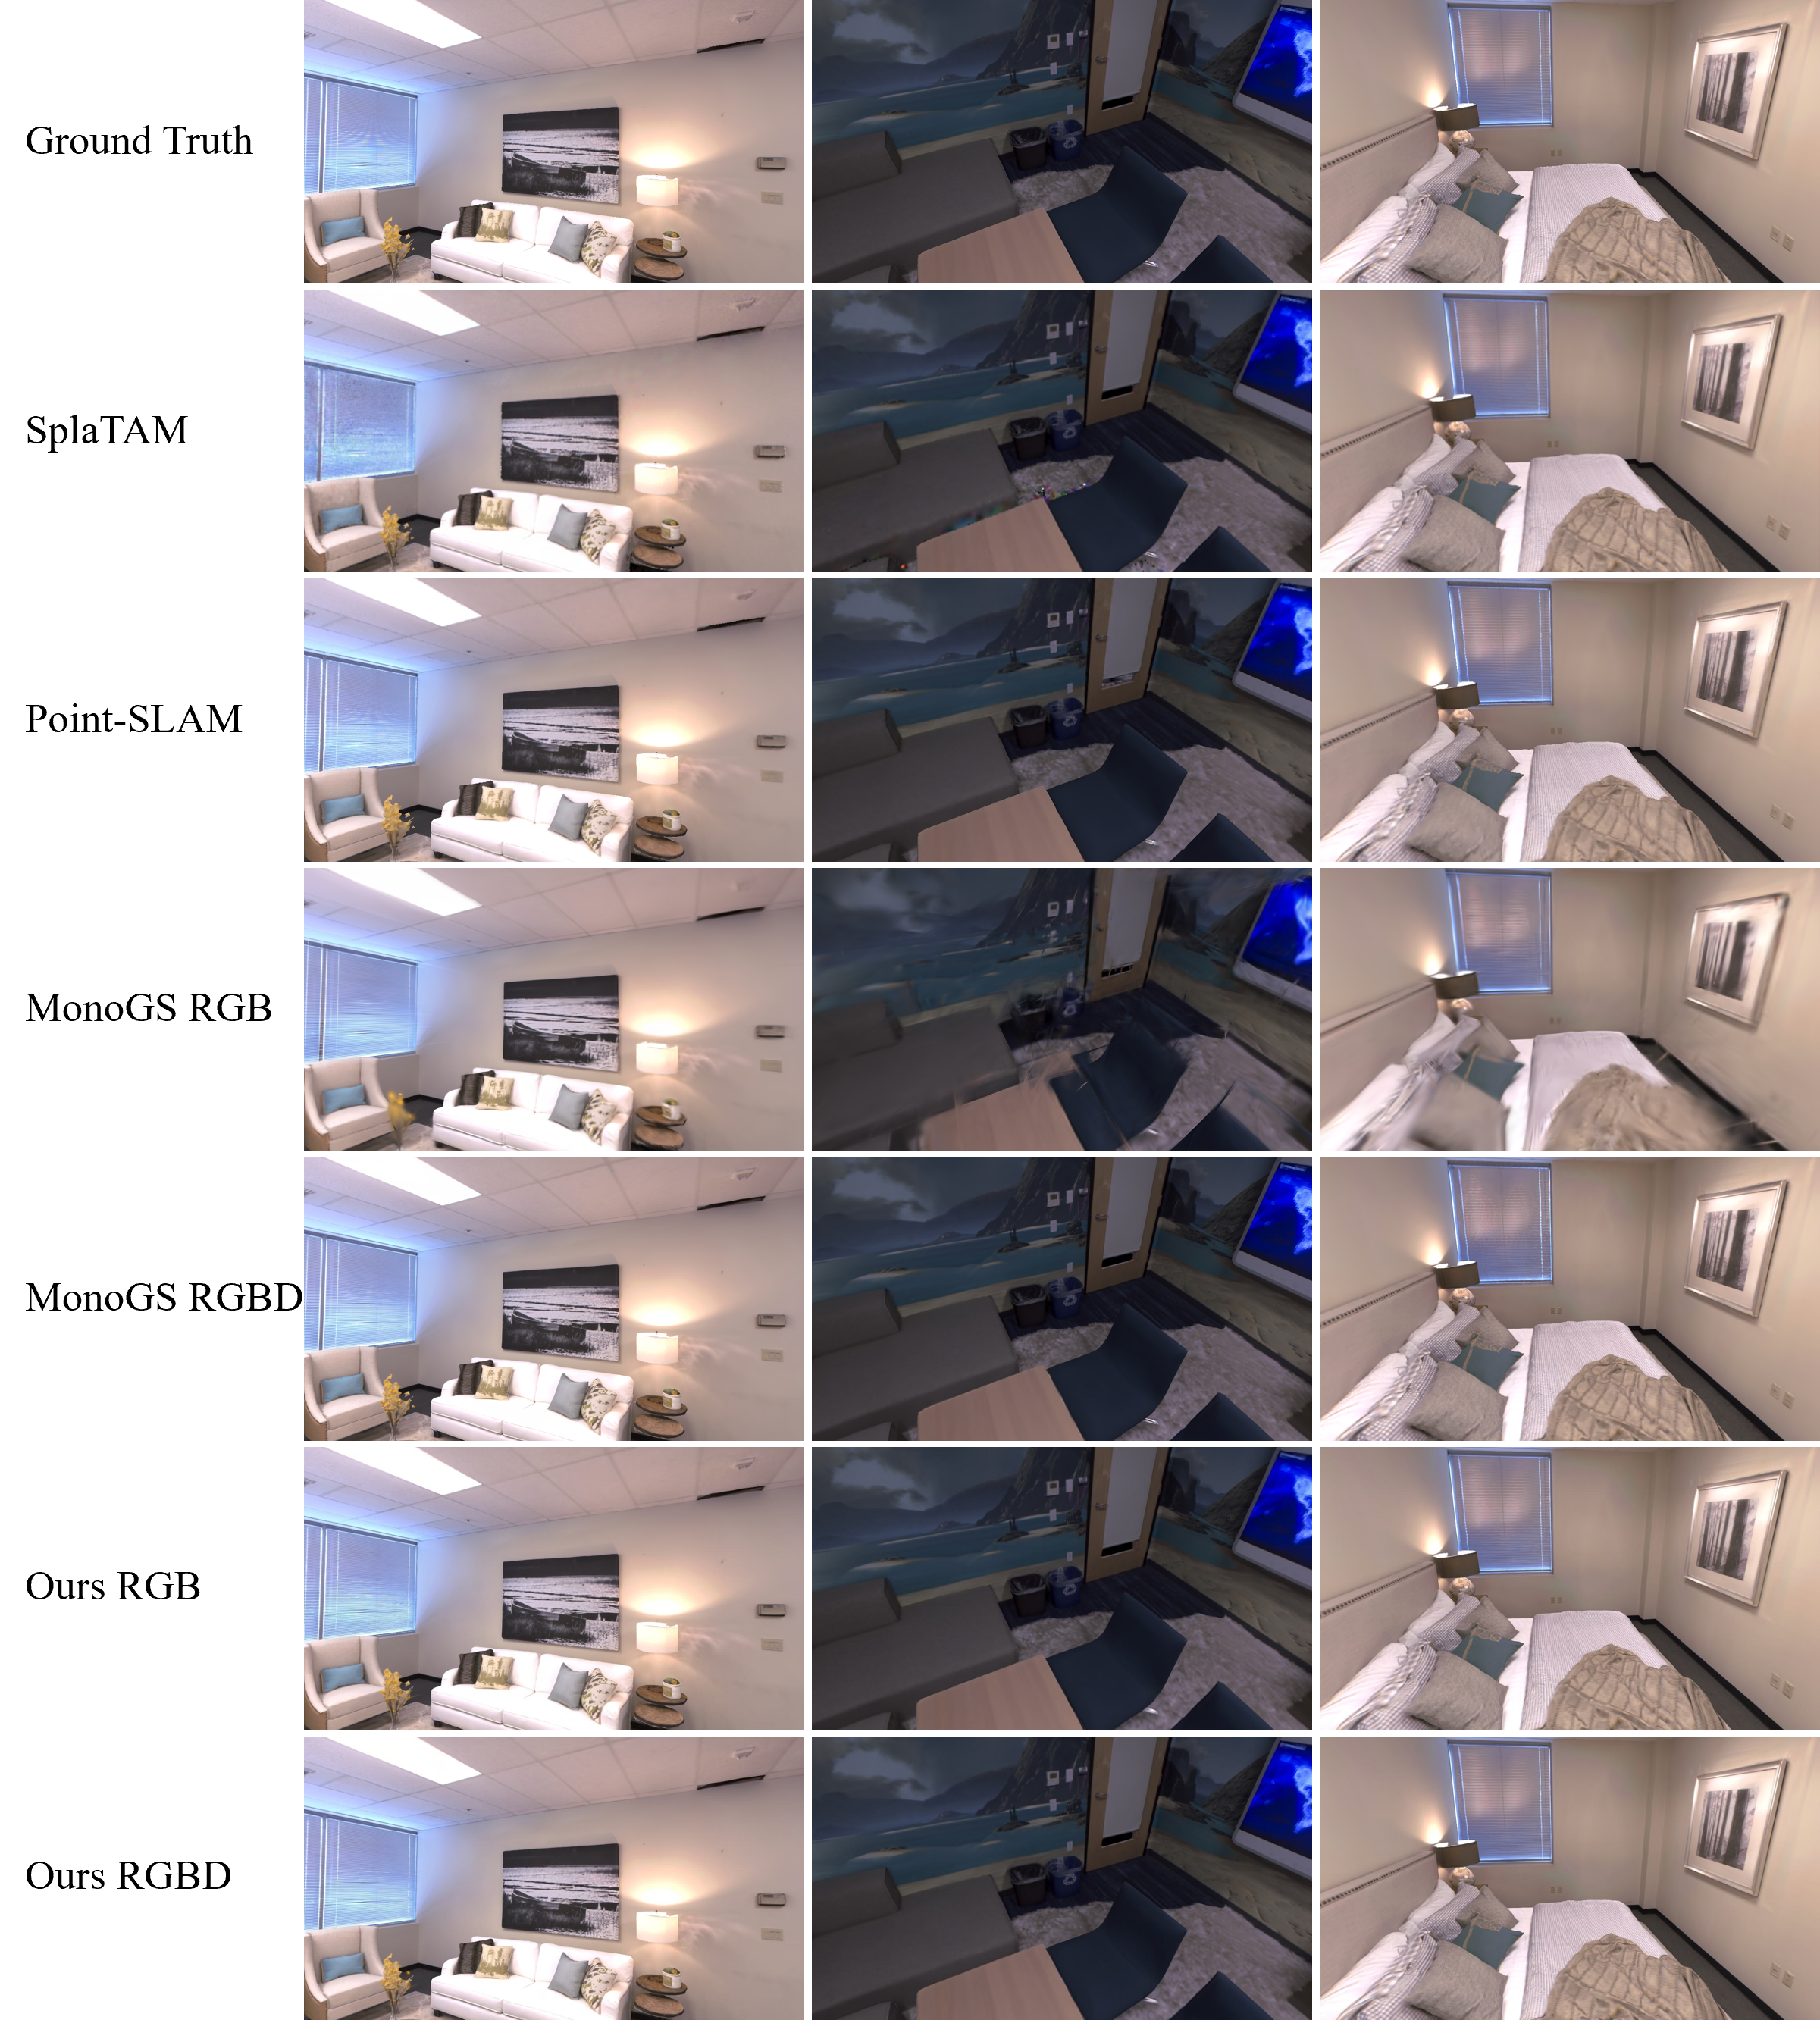}
    \caption{Rendering samples on Replica dataset.}
    \label{fig:fig_supp_fig2}
\end{figure*}
