# Supplementary material for: MonoGS++: Fast and Accurate Monocular RGB Gaussian SLAM
Source: arXiv:2504.02437 source file (2025-04-03)
Supplement: Supplementary file 6 [file supp_memory.tex]

\begin{table}[htbp]
    \centering
    \resizebox{0.65\textwidth}{!}{
    \begin{tabular}{cccc}
    \hline
      Method          &  SplaTAM~\cite{splatam} & MonoGS~\cite{monogs} & Ours \\ \hline
      GPU Memory (MB)    &  11611 & 15315 & 8104 \\ \hline    
    \end{tabular}
    }
    \caption{\textbf{GPU memory consumption comparison.} We compare GPU memory consumption with baselines SplaTAM~\cite{splatam} and MonoGS~\cite{monogs} on Replica/room0.}
    \label{tab:tab:memory}
\end{table}
